# Supplementary material for: Read-Rezayi fractional Chern insulators in modulated Bernal graphene
Source: arXiv:2609.31846 source file (2026-12-01)
Supplement: Supplementary file 1 [file supp-setup.tex]

%-----EXTERNAL DOCUMENT FOR CROSS-REFERENCING-----
\usepackage{xr}
\makeatletter
\newcommand*{\addFileDependency}[1]{% argument=file name and extension
  \typeout{(#1)}% latexmk will find this if $recorder=0 (however, in that case, it will ignore #1 if it is a .aux or .pdf file etc and it exists! if it doesn't exist, it will appear in the list of dependents regardless)
  \@addtofilelist{#1}% if you want it to appear in \listfiles, not really necessary and latexmk doesn't use this
  \IfFileExists{#1}{}{\typeout{No file #1.}}% latexmk will find this message if #1 doesn't exist (yet)
}
\makeatother

\newcommand*{\myexternaldocument}[1]{%
    \externaldocument{#1}%
    \addFileDependency{#1.tex}%
    \addFileDependency{#1.aux}%
}

%-----PACKAGES-----
\usepackage[pdftex]{hyperref}
\hypersetup{
  colorlinks,
	linkcolor={blue!75!black!80!yellow},
	citecolor={blue!75!black!80!yellow},
	urlcolor={blue!75!black!80!yellow},
	pdfstartview=FitH,
	}
\usepackage[top=1in, bottom=1.5in, left=1.25in, right=1.25in]{geometry} %Change margins
\usepackage{graphicx}
\usepackage{xspace}
\newcommand\bmmax{0} % the bm package takes up a lot of alphabets internally, making it impossible to load more font packages (like sansmath); reduce the number of preloaded alphabets to avoid this
\usepackage{bm}
\usepackage[usenames,dvipsnames]{xcolor}
%\usepackage[only, llbracket, rrbracket]{stmaryrd} % provides \llbracket and \rrbracket for difference-operations
\usepackage[UKenglish]{babel}
\usepackage{enumitem} % allows changing enumerate bullets
\usepackage{multirow}

\usepackage[perpage, symbol*, hang, multiple]{footmisc} % avoid footnote-counter trouble when using footnote symbols rather than numbers
\setfnsymbol{lamport} % footmisc's symbol* option fails if we don't set this explicitly somehow
\renewcommand{\footnotemargin}{.85em}
\setlength{\footnotesep}{.65\baselineskip}
\renewcommand{\hangfootparskip}{0.15\baselineskip}
%\renewcommand\thefootnote{\fnsymbol{footnote}}

%-----SI UNITS-----
\usepackage{siunitx}
\sisetup{range-phrase =\text{\,--\,},
	list-units   =single,
	range-units  =single,
	list-pair-separator = {\ \text{and}\ },
	list-separator = {,\ \linebreak[0]},
	list-final-separator = {,\ \linebreak[0]\text{and}\ },
    group-separator = {\,},
    detect-all = true
}
\DeclareSIUnit[number-unit-product = ]\percent{\char`\%} % remove spacing for \percent

%-----APPPEND 'S' TO REFERENCES OF ALL KINDS-----
\renewcommand{\theequation}{S\arabic{equation}} %Equations
\renewcommand{\thefigure}{S\arabic{figure}} %Figures
\renewcommand{\thetable}{S\arabic{table}} %Tables
\renewcommand{\bibnumfmt}[1]{[S#1]} %Citations
\renewcommand{\citenumfont}[1]{S#1}
\renewcommand*\descriptionlabel[1]{\hspace\labelsep\normalfont\itshape #1\ \hfil} %Change appearance of description lists

%-----LOADING RELEVANT FONTS [Times Roman]-----
\usepackage{txfonts}  %Times Roman fonts
\usepackage{txfontsb} %Addition for txfonts, including old style numerals and greek
\usepackage{microtype} %For better kerning and symbol-stretching

%-----REDEFINE THE RMP STYLE OF AUTHORS AND AFFILIATIONS-----
\makeatletter
\def\frontmatter@authorformat{%
	\preprintsty@sw{\vskip0.5pc\relax}{}%
	\@tempskipa\@flushglue
	\@flushglue\z@ plus50\p@\relax
	\raggedright\advance\leftskip.25in\relax
	\@flushglue\@tempskipa
	\parskip\z@skip
}%
%
\def\frontmatter@affiliationfont{% Helvetica 9/10.2
	\small\slshape\selectfont\baselineskip10.5\p@\relax
	\@tempskipa\@flushglue
	\@flushglue\z@ plus50\p@\relax
	\raggedright\advance\leftskip.25in\relax
	\@flushglue\@tempskipa
}
%	
\def\paragraph{%
	\@startsection
	{paragraph}%
	{4}%
	{\parindent}%
	{\z@}%
	{-1em}%
	{\normalfont\small\itshape\textsf}%%Change so that paragraphs are also in sans serif font
}%
\renewcommand*\email[1][]{\begingroup\sanitize@url\@email{#1}} %Remove the 'Electronic adress: ' from RMP style
\makeatother

\setcitestyle{numbers,square,sort&compress} %We don't want the rmp citation style, but standard style square bracket, numbers style instead

% Section numbering
\renewcommand{\thesection}{S\arabic{section}}
\renewcommand{\thesubsection}{\Alph{subsection}}
\renewcommand{\thesubsubsection}{\roman{subsubsection}}

% 

%----- Changes to caption -----
% These hacks are specific to revtex4 (and maybe 4-2?) (revtex4-1 solution doesn't work)
\usepackage{braket}
\usepackage[EULERGREEK]{sansmath}
\makeatletter 
% set caption title to bold sans serif... 
\renewcommand*{\fnum@figure}{{\sffamily\bfseries{}Supplemental Figure~\thefigure{}.}}  % figure caption title
\renewcommand*{\fnum@table}{{\sffamily\bfseries{}Supplemental Table~\thetable{}.}}     % table caption title
\newcommand{\supptablename}{\fnum@table}

% set all caption contents to sans serif
\long\def\@makecaption#1#2{%
  \vskip\abovecaptionskip
  \vbox{%
   \flushing%
   \sisetup{math-sf=\textsf}%
   \small\sffamily\sansmath%
   \noindent
   #1\nobreak\hskip.5em plus.2em\ignorespaces#2\par
  }%
  \vskip\belowcaptionskip
}%

% Hack to change section name of references to all-caps Supplemental references while keeping
% table-of-contents reference lower case.
\newcommand{\nocontentsline}[3]{}
\newcommand{\tocless}[2]{\bgroup\let\addcontentsline=\nocontentsline#1{#2}\egroup}
\def\bibsection{%
 \@ifx@empty\refname{%
  \par
 }{%
  \let\@hangfroms@section\@hang@froms
  \phantomsection
  \addcontentsline{toc}{section}{Supplemental References}
  \tocless{\section*{SUPPLEMENTAL REFERENCES}}%
  \@nobreaktrue
 }%
}%
\makeatother

%----- Spacing and binary relations/operations -----
\thickmuskip=5mu plus 2mu minus 1mu  %binary relations (default, 5mu plus 5mu)
\medmuskip=4mu plus 2mu minus 2mu    %binary operations (default, 4mu plus 2mu minus 4mu)
\frenchspacing %Ensure that revTeX does not do "double spaces" after punctuation

%-----Changing appearance of ToC-----
\makeatletter
    \DeclareRobustCommand*{\deactivateaddvspace}{\let\addvspace\@gobble} % "deactivates" \addvspace command
    \DeclareRobustCommand*{\deactivatetocsubsections}{
    \def\l@subsection##1##2{}    % these definitions are inherited from \l@@sections, see 
    \def\l@subsubsection##1##2{} % ltxutils.dtx; "reset" them to remove subsections in ToC
    }
\makeatother

%-----PACKAGE TO ALLOW A \FloatBarrier TO FORCE EXECUTION OF FLOATS-----
\usepackage{placeins}

%-----COMMANDS-----
\input{commands.tex}

% commands specific to look of computer-generated tables
\newcommand{\msf}[1]{\mbox{\sansmath$\mathsf{#1}$}} % clash between mathsf and sansmath, fix via https://tex.stackexchange.com/a/172862/113831
\newcommand{\mmsf}[1]{#1}
\newcommand{\tT}{^{\scalebox{.8}{2T}}}
\newcommand{\tToL}{^{\scalebox{.8}{2T+1L}}}
\newcommand{\oT}{^{\scalebox{.8}{T}}}


%-----COMMENTS AND META-ANNOTATIONS-----
\usepackage{textcomp} % for \textrightarrow
\usepackage{xifthen}
\usepackage{etoolbox}
\newboolean{togglecomments}
\newboolean{togglechanges} 

% toggle to true to see comments (otherwise hidden)
\setboolean{togglecomments}{true}  
% toggle to false to see mixed versions (otherwise edits are shown exclusively)
\setboolean{togglechanges}{false} 

\newcommand{\textblacksquare}{$\blacksquare$}
\newcommand{\todo}[1]{\ifbool{togglecomments}%
	{\textcolor{green!60!black}{\small\textsf{{}\textsuperscript{\textsc{\textsf{todo}}}}[#1]}} % if true, show comments
	{}}     % if false, do nothing
\newcommand{\comment}[2]{\ifbool{togglecomments}%
		{\textcolor{blue!70!black}{\small\sf\textsuperscript{\textsc{\textsf{#1}}}[#2]}} % if true, show comments
		{}}     % if false, do nothing

\newcommand{\commentAGF}[1]{\ifbool{togglecomments}%
		{\textcolor{red!70!black}{\small\sf\textsuperscript{\textsc{\textsf{\ignorespaces AGF}}}[\ignorespaces#1]}} % if true, show comments
		{}}     % if false, do nothing

\newcommand{\commentRMS}[1]{\ifbool{togglecomments}%
		{\textcolor{violet!70!black}{\small\sf\textsuperscript{\textsc{\textsf{\ignorespaces RMS}}}[\ignorespaces#1]}} % if true, show comments
		{}}   
    
\newcommand{\swap}[2]{\ifbool{togglechanges}
	{#2}  % revisions-only version
	{\textcolor{red!70!black}{[#1]}\textrightarrow{}\textcolor{green!50!black}{[#2]}}}
\newcommand{\remove}[1]{\ifbool{togglechanges}
	{}    % revisions-only version
	{\textcolor{red!70!black}{#1}}}
\newcommand{\inset}[1]{\ifbool{togglechanges}
	{#1}  % revisions-only version
	{\textcolor{green!50!black}{#1}}}
\newcommand{\citeremind}[1]{%
	[\textcolor{blue!75!black!80!yellow}{\textblacksquare%
		\ifthenelse{\isempty{#1}}{}{\textsuperscript{\tiny\textsf{#1}}}%
	}]\xspace}
\newcommand{\fixme}[1]{\textcolor{red!70!black}{[#1]}}
\newcommand{\optional}[1]{\textcolor{orange!70!gray}{#1}}
    
%-----REFERENCING VIA CLEVEREF-----
\usepackage[capitalize,nameinlink]{cleveref}
\newcommand{\crefrangeconjunction}{\,--\,}
\crefname{subequations}{Eqs.}{Eqs.} %Specific changes to allow for Eqs.-wording when referring to a set of subequations. Label of subequations must include [subequations] as an option.
\Crefname{subequations}{Eqs.}{Eqs.}
\crefformat{subequations}{#2Eqs.~(#1)#3}
\Crefformat{subequations}{#2Eqs.~(#1)#3}
\crefname{page}{p.}{p.} %Changing from 'page' to 'p.'
\crefname{table}{Table}{Tables}
\crefname{figure}{Figure}{Figures}
\crefname{section}{Section}{Sections}

%-----LONGTABLE PACKAGE AND WRAPPERS----
\usepackage{longtable, booktabs}
\usepackage{floatrow}
\floatsetup[table]{font={sf}}
\usepackage{colortbl} % to change color of e.g. \midrule
\usepackage{adjustbox}
\usepackage{colortbl}
\newcommand{\separatorrule}{\arrayrulecolor{black!25}\specialrule{.25pt}{.65\jot}{.65\jot}\arrayrulecolor{black}}

%-----CUSTOM COLORS-----
\definecolor{tred}{RGB}{214, 48, 49}
\definecolor{tblue}{RGB}{9, 132, 227}
\definecolor{tgreen}{RGB}{39, 174, 96}

%-----JULIA CODE LISTINGS-----
\usepackage{listings}

\lstdefinelanguage{Julia}%
  {morekeywords={abstract,break,case,catch,const,continue,do,else,elseif,%
   end,export,false,for,function,mutable,struct,import,if,in,%
   macro,module,otherwise,quote,return,switch,try,type,%
   using,while},%
   sensitive=true,%
   alsoother={$},%
   morecomment=[l]\#,%
   morecomment=[n]{\#=}{=\#},%
   morestring=[s]{"}{"},%
   morestring=[m]{'}{'},%
}[keywords,comments,strings]%

\lstset{%
    language         = Julia,
    basicstyle       = \small\ttfamily,
    keywordstyle     = \bfseries,
    stringstyle      = \color{magenta},
    commentstyle     = \color{ForestGreen},
    showstringspaces = false,
    inputencoding	 = utf8,
    extendedchars	 = true,
    xleftmargin 	 = .25in,
    literate=
        {¹}{{\textsuperscript{1}}}1 {ᴸ}{{\textsuperscript{L}}}1 {ᵀ}{{\textsuperscript{T}}}1
        {ⁱ}{{\textsuperscript{i}}}1
        {⁺}{{$^+$}}1 {⁻}{{$^-$}}1 
        {₁}{{\textsubscript{1}}}1 {₂}{{\textsubscript{1}}}1 {₃}{{\textsubscript{3}}}1 {₄}{{\textsubscript{4}}}1
        {Γ}{{$\Gamma$}}1
}
